# Supplementary material for: TorchEsegeta: Framework for Interpretability and Explainability of Image-based Deep Learning Models
Source: arXiv:2110.08429 source file (2022-02-07)
Supplement: Supplementary file 1 [file 4_2_additional_results.tex]

%--- old results
% \newpage
% \par
% 1. CNN Visualization Integrated Gradient
% \newline
% \hfill \break
% Attribution Image for 3 models
% \newline
%     \begin{minipage}[t]{7cm}
% 			 \centering
% 			 \includegraphics[width=9cm, height=4cm]{images/cnnvisig_ig_attri.PNG}
%   \end{minipage}
%   \par
   
%   CNN Visualization Integrated Gradient attribution zoomed images:
%   \hfill \break
%   \par
%   \begin{minipage}[t]{7cm}
% 			 \centering
% 			 \includegraphics[width=9cm,height=4cm]{images/cnnvis_ig_mssdef_zoom.PNG}
%   \end{minipage}
%   \par
%       \hfill \break
%   \begin{minipage}[t]{7cm}
% 			 \centering
% 			 \includegraphics[width=9cm,height=4cm]{images/cnnvis_ig_mssdef_zoom.PNG}
%   \end{minipage}
%   \par
%       \hfill \break
%   \begin{minipage}[t]{7cm}
% 			 \centering
% 			 \includegraphics[width=9cm,height=4cm]{images/cnnvis_ig_unet_zoomed.PNG}
%   \end{minipage}
  
% \vspace{60mm}
% 2. Captum Saliency
% \newline
% \hfill \break
%  Attribution Image for 3 models
%  \newline
%   \begin{minipage}[t]{7cm}
% 			 \centering
% 			 \includegraphics[width=9cm, height=4cm]{images/captumsaliency_attr.PNG}
%   \end{minipage}
% \par

%       Captum Saliency attribution zoomed images:
%   \hfill\break      
%   \par
%   \begin{minipage}[t]{7cm}
% 			 \centering
% 			 \includegraphics[width=9cm, height=4cm]{images/captumsalieny_unetmssdef_zoom.PNG}
%   \end{minipage}
%   \hfill \break
%   \par
%   \begin{minipage}[t]{7cm}
% 			 \centering
% 			 \includegraphics[width=9cm, height=4cm]{images/captumsalieny_unetmss_zoom.PNG}
%   \end{minipage}
%   \hfill \break
%   \par
%   \begin{minipage}[t]{7cm}
% 			 \centering
% 			 \includegraphics[width=9cm, height=4cm]{images/captumsalieny_unet_zoom.PNG}
%   \end{minipage}
%   \par
%   \vspace{60mm}
% 3. Captum Deconvolution
% \newline
% \hfill\break
%  Attribution Image for 3 models
%  \newline
%   \begin{minipage}[t]{7cm}
% 			 \centering
% 			 \includegraphics[width=9cm, height=4cm]{images/captumdeconv_attr.PNG}
%   \end{minipage}
%   \par
   
%   Captum Deconvolution attribution zoomed images
%     \hfill\break
%     \par
%       \begin{minipage}[t]{7cm}
% 			 \centering
% 			 \includegraphics[width=9cm,height=4cm]{images/captumdeconv_unetmssdeform.PNG}
%   \end{minipage}
%   \hfill\break
%   \par
%       \begin{minipage}[t]{7cm}
% 			 \centering
% 			 \includegraphics[width=9cm,height=4cm]{images/captumdeconv_unetmss.PNG}
%   \end{minipage}
%   \hfill\break
%   \par
%       \begin{minipage}[t]{7cm}
% 			 \centering
% 			 \includegraphics[width=9cm,height=4cm]{images/captumdeconv_unet.PNG}
%   \end{minipage}
%   \par
%   \vspace{60mm}
% 4. Captum Guided Backprop
% \newline
% \hfill\break
%  Attribution Image for 3 models
%  \newline
%   \begin{minipage}[t]{7cm}
% 			 \centering
% 			 \includegraphics[width=9cm, height=4cm]{images/Captumgbp_attr.PNG}
%   \end{minipage}
%   \par
%   Captum Guided Backprop attribution zoomed images
%   \par
%   \begin{minipage}[t]{7cm}
% 			 \centering
% 			 \includegraphics[width=9cm,height=4cm]{images/captumgbp_unetmssdef.PNG}
%   \end{minipage}
%   \hfill\break
%   \par
   
%   \begin{minipage}[t]{7cm}
% 			 \centering
% 			 \includegraphics[width=9cm,height=4cm]{images/captumgbp_unetmss_zoom.PNG}
%   \end{minipage}
%   \hfill\break
%   \par
   
%   \begin{minipage}[t]{7cm}
% 			 \centering
% 			 \includegraphics[width=9cm,height=4cm]{images/captumgbp_unet_zoom.PNG}
%   \end{minipage}
%   \par
%   \vspace{60mm}
% 5. CNN Visualization Layer activation Guided Backpropagation
% \newline
% \hfill\break
%  Attribution Image for 3 models
%  \newline
%   \begin{minipage}[t]{7cm}
% 			 \centering
% 			 \includegraphics[width=9cm,height=4cm]{images/cnnvis_layeractigbp_attr.PNG}
%   \end{minipage}
%   \par
%   CNN Visualization Layer activation Guided Backpropagation attribution zoomed images
%   \hfill\break
%   \par
%       \begin{minipage}[t]{7cm}
% 			 \centering
% 			 \includegraphics[width=9cm,height=4cm]{images/cnnvis_layeractigbp_unetmssdef_zoom.PNG}
%   \end{minipage}
%   \hfill\break
%   \par
%       \begin{minipage}[t]{7cm}
% 			 \centering
% 			 \includegraphics[width=9cm,height=4cm]{images/cnnvis_layeractigbp_unetmss_zoom.PNG}
%   \end{minipage}
%   \hfill\break
%   \par
%       \begin{minipage}[t]{7cm}
% 			 \centering
% 			 \includegraphics[width=9cm,height=4cm]{images/cnnvis_layeractigbp_unet_zoom.PNG}
%   \end{minipage}
%   \par
%   \vspace{60mm}
% 6. TorchRay Deconv
%   \newline
%   \hfill\break
%     Attribution Image for 3 models
%  \newline
%       \begin{minipage}[t]{7cm}
% 			 \centering
% 			 \includegraphics[width=9cm,height=4cm]{images/tochray_deconv_attr.JPG}
%   \end{minipage}
   
%       \par
      
%       TorchRay Deconv attribution zoomed images
%       \hfill\break
%       \par
%       \begin{minipage}[t]{7cm}
% 			 \centering
% 			 \includegraphics[width=9cm,height=4cm]{images/tochraydeconv_deform_zoom.JPG}
%   \end{minipage}
%   \hfill\break
%   \par
   
%       \begin{minipage}[t]{7cm}
% 			 \centering
% 			 \includegraphics[width=9cm,height=4cm]{images/tochraydeconv_mss_zoom.JPG}
%   \end{minipage}
%   \hfill\break
%   \par
   
%       \begin{minipage}[t]{7cm}
% 			 \centering
% 			 \includegraphics[width=9cm,height=4cm]{images/tochraydeconv_unet_zoom.JPG}
%   \end{minipage}
%   \par
%   \vspace{60mm}
%   \newpage
%       Comparison of different outputs for captum based methods:
%   \par
%       \begin{minipage}[t]{7cm}
% 			 \centering
% 			 \includegraphics[width=18cm]{images/captum_method_comap.PNG}
%   \end{minipage}
% \par
% \clearpage
% \par


% Captum Saliency:

% The image shows the cascading of the network starting from the very last layer. The caption Cascading Random 1 is the output obtained after randomising the weights of just the last layer of the network and obtaining the output from the Captum Saliency method. Compared to the original output of the Saliency method, the cascaded output has very few activations suggesting that the output of the method is largely dependent on the network weights. As we further cascade above layers and observe the output, almost all the cascaded images have no activations asserting the fact that the output for this method is dependent mainly on network weights. 
% \par
%   \begin{minipage}[t]{7cm}
% 			 \centering
% 			 \includegraphics[width=9cm,height=8cm]{images/captumsailency_cascade1-9.PNG}
%   \end{minipage}
%   \par
%       \begin{minipage}[t]{7cm}
% 			 \centering
% 			 \includegraphics[width=9cm,height=8cm]{images/captumsaliency_cascade10-18.PNG}
%   \end{minipage}

% \par
% \newpage
% CNN Visualization Integrated Gradients:

% Similar comparisons can be drawn for Integrated gradients as that of Saliency. However, none of the cascaded images of Integrated gradients has any activations, which again suggests that the method's output has a very high dependency on each layer of the network. Another hypothesis that can be proposed is that the output for this method is strongly dependent on the last layer of the network, and randomising that at the very beginning also affects the outputs of the other layers concurrently. 
% \par
%       \begin{minipage}[t]{7cm}
% 			 \centering
% 			 \includegraphics[width=9cm,height=8cm]{images/cnnvis_ig_cascade1-9.PNG}
%   \end{minipage}
% \par
%       \begin{minipage}[t]{7cm}
% 			 \centering
% 			 \includegraphics[width=9cm,height=8cm]{images/cnnvis_ig_cascade10-18.PNG}
%   \end{minipage}
%   \par
%---- old results------------



%\chapter{Anhänge}
% \vspace{100mm}
% \subsection{Additional Results}
% \label{c:cs}
% \unitlength1mm
% 1. Captum Guided Grad CAM Attribution
% \newline
% \hfill\break

%   \begin{minipage}[t]{7cm}
% 			 \centering
% 			 \includegraphics[width=9cm, height=4cm]{images/captumggc_attr.PNG}
%   \end{minipage}
%   \par
%   Captum Guided Grad CAM Attribution Zoomed Images
%   \par
%       \begin{minipage}[t]{7cm}
% 			 \centering
% 			 \includegraphics[width=9cm,height=4cm]{images/captumggc_unetmssdef_zoom.PNG}
%   \end{minipage}
%   \hfill\break
%   \par
%          \begin{minipage}[t]{7cm}
% 			 \centering
% 			 \includegraphics[width=9cm,height=4cm]{images/captumggc_unetmss_zoom.PNG}
%   \end{minipage}
%   \hfill\break
%   \par
%          \begin{minipage}[t]{7cm}
% 			 \centering
% 			 \includegraphics[width=9cm,height=4cm]{images/captumggc_unet_zoom.PNG}
%   \end{minipage}
%   \hfill\break
%   \par
%   \vspace{60mm}
%   CNN Visualization Guided Backpropagation Attribution
% \newline
% \hfill\break
%          \begin{minipage}[t]{7cm}
% 			 \centering
% 			 \includegraphics[width=9cm,height=4cm]{images/cnnvis_gbp_attri.PNG}
%   \end{minipage}
%   \par
   
%       CNN Visualization Guided Backpropagation Attribution zoomed images
%       \par
%           \begin{minipage}[t]{7cm}
% 			 \centering
% 			 \includegraphics[width=9cm,height=4cm]{images/cnnvis_gbp_unetmssdef_zoom.PNG}
%   \end{minipage}
%   \hfill\break
%   \par
%           \begin{minipage}[t]{7cm}
% 			 \centering
% 			 \includegraphics[width=9cm,height=4cm]{images/cnnvis_gbp_unetmss_zoom.PNG}
%   \end{minipage}
%   \hfill\break
%   \par
%           \begin{minipage}[t]{7cm}
% 			 \centering
% 			 \includegraphics[width=9cm,height=4cm]{images/cnnvis_gbp_unet_zoom.PNG}
%   \end{minipage}
%   \par
%   \vspace{60mm}
% CNN Visualization Guided Grad CAM Attribution
% \newline
% \hfill\break
%             \begin{minipage}[t]{7cm}
% 			 \centering
% 			 \includegraphics[width=9cm,height=4cm]{images/cnnvisggc_attr.PNG}
%   \end{minipage}
%   \par
%       CNN Visualization Guided Grad CAM Attribution zoomed images
%       \par
%               \begin{minipage}[t]{7cm}
% 			 \centering
% 			 \includegraphics[width=9cm,height=4cm]{images/cnnvisggc_unetmssdef_zoom.PNG}
%   \end{minipage}
%   \hfill\break
%   \par
%                  \begin{minipage}[t]{7cm}
% 			 \centering
% 			 \includegraphics[width=9cm,height=4cm]{images/cnnvisggc_unetmss_zoom.PNG}
%   \end{minipage}
%   \hfill\break
%   \par
%                  \begin{minipage}[t]{7cm}
% 			 \centering
% 			 \includegraphics[width=9cm,height=4cm]{images/cnnvisggc_unet_zoom.PNG}
%   \end{minipage}
%   \hfill\break
%   \par
%   \vspace{60mm}
% CNN Visualization Grad CAM Attribution
%          \par
%                  \begin{minipage}[t]{7cm}
% 			 \centering
% 			 \includegraphics[width=9cm, height=4cm]{images/cnnvis_gradcam_attr.JPG}
%   \end{minipage}
%   \par
%   \hfill\break
% CNN Visualization Grad Times Image Attribution
%             \par
%                  \begin{minipage}[t]{7cm}
% 			 \centering
% 			 \includegraphics[width=9cm,height=4cm]{images/cnnvis_gradtimesimage_attr.JPG}
%   \end{minipage}
%   \par
%   \hfill\break
% CNN Visualization Vanilla Backpropagation Attribution
%              \par
%                  \begin{minipage}[t]{7cm}
% 			 \centering
% 			 \includegraphics[width=9cm,height=4cm]{images/cnnvis_vaillabackrop_attr.JPG}
%   \end{minipage}
%   \par
